# Supplementary material for: Localized, High-resolution Geographic Representations with Slepian Functions
Source: arXiv:2602.00392 source file (2026-06-02)
Supplement: Supplementary file 1 [file shannon_number.tex]

\definecolor{shL10}{RGB}{31,119,180}
\definecolor{shL20}{RGB}{255,127,14}
\definecolor{shL30}{RGB}{44,160,44}
\definecolor{shL40}{RGB}{214,39,40}
\definecolor{slepL60}{RGB}{31,119,180}
\definecolor{slepL80}{RGB}{255,127,14}
\definecolor{slepL120}{RGB}{44,160,44}
\definecolor{slepL200}{RGB}{214,39,40}

\begin{wrapfigure}{r}{0.6\textwidth}
    \centering
    \begin{tikzpicture}
        % Common Y label
        \node[rotate=90, anchor=south, font=\small] at (-0.4, 1.9) {$R^2$};
        
        % Left plot: Slepian (log scale to spread early dims)
        \begin{axis}[
            name=slepian,
            width=0.55\linewidth,
            height=4cm,
            xlabel={Embedding Size},
            ylabel={},
            title={\textbf{(a)} Slepian},
            % xmode=log,
            xmin=1.5, xmax=110,
            ymin=0.35, ymax=0.72,
            grid=major,
            grid style={line width=0.1pt, draw=gray!20},
            tick label style={font=\scriptsize},
            label style={font=\scriptsize},
            title style={font=\small, yshift=-0.5ex},
            legend style={font=\tiny, at={(0.98,0.02)}, anchor=south east, cells={anchor=west}, row sep=-2pt},
            mark size=1.2pt,
            line width=0.8pt,
        ]
        
        % Shannon number vertical lines (dashed)
        \addplot[dashed, color=slepL60, line width=0.6pt, forget plot] coordinates {(7, 0.35) (7, 0.72)};
        \addplot[dashed, color=slepL80, line width=0.6pt, forget plot] coordinates {(12, 0.35) (12, 0.72)};
        \addplot[dashed, color=slepL120, line width=0.6pt, forget plot] coordinates {(28, 0.35) (28, 0.72)};
        \addplot[dashed, color=slepL200, line width=0.6pt, forget plot] coordinates {(77, 0.35) (77, 0.72)};
        
        % L=60 data (Shannon ~7)
        \addplot[color=slepL60, mark=*, mark options={solid, fill=slepL60}] coordinates {
            (2, 0.392) (4, 0.495) (6, 0.555) (9, 0.563) (12, 0.571) (14, 0.584)
        };
        \addlegendentry{$L=60$}
        
        % L=80 data (Shannon ~12)
        \addplot[color=slepL80, mark=square*, mark options={solid, fill=slepL80}] coordinates {
            (2, 0.397) (4, 0.499) (6, 0.547) (11, 0.581) (14, 0.588) (15, 0.605) (21, 0.598)
        };
        \addlegendentry{$L=80$}
        
        % L=120 data (Shannon ~28)
        \addplot[color=slepL120, mark=triangle*, mark options={solid, fill=slepL120}] coordinates {
            (2, 0.405) (4, 0.485) (6, 0.535) (9, 0.584) (21, 0.625) (26, 0.635) (29, 0.643) (35, 0.634) (41, 0.650)
        };
        \addlegendentry{$L=120$}
        
        % L=200 data (Shannon ~77)
        \addplot[color=slepL200, mark=diamond*, mark options={solid, fill=slepL200}] coordinates {
            (2, 0.434) (4, 0.479) (6, 0.502) (13, 0.577) (19, 0.599) (28, 0.630) (42, 0.657) (63, 0.670) (75, 0.671) (84, 0.679) (98, 0.674)
        };
        \addlegendentry{$L=200$}
        
        \end{axis}
        
        % Right plot: Vanilla SH
        \begin{axis}[
            at={(slepian.east)},
            anchor=west,
            xshift=0.4cm,
            width=0.50\linewidth,
            height=4cm,
            xlabel={Embedding Size},
            ylabel={},
            title={\textbf{(b)} Spherical Harmonics},
            xmin=0, xmax=420,
            ymin=0, ymax=0.6,
            grid=major,
            grid style={line width=0.1pt, draw=gray!20},
            tick label style={font=\scriptsize},
            label style={font=\scriptsize},
            title style={font=\small, yshift=-0.5ex},
            legend style={font=\tiny, at={(0.98,0.02)}, anchor=south east, cells={anchor=west}, row sep=-2pt},
            mark size=1.2pt,
            line width=0.8pt,
        ]
        
        % L=10 data
        \addplot[color=shL10, mark=*, mark options={solid, fill=shL10}] coordinates {
            (2, 0.007) (4, 0.310) (8, 0.316) (16, 0.324) (24, 0.370)
            (32, 0.370) (48, 0.382) (64, 0.382) (80, 0.392) (100, 0.401)
        };
        \addlegendentry{$L=10$}
        
        % L=20 data
        \addplot[color=shL20, mark=square*, mark options={solid, fill=shL20}] coordinates {
            (2, 0.007) (4, 0.291) (16, 0.348) (32, 0.380) (64, 0.396)
            (96, 0.385) (128, 0.386) (192, 0.415) (256, 0.428) (272, 0.397) (320, 0.457) (400, 0.497)
        };
        \addlegendentry{$L=20$}
        
        % L=30 data
        \addplot[color=shL30, mark=triangle*, mark options={solid, fill=shL30}] coordinates {
            (2, 0.007) (16, 0.331) (48, 0.386) (96, 0.377) (144, 0.410)
            (192, 0.403) (272, 0.471) (368, 0.488) (400, 0.466)
        };
        \addlegendentry{$L=30$}
        
        % L=40 data
        \addplot[color=shL40, mark=diamond*, mark options={solid, fill=shL40}] coordinates {
            (2, 0.006) (16, 0.338) (48, 0.382) (96, 0.387) (144, 0.404)
            (208, 0.435) (336, 0.452) (384, 0.481) (400, 0.426)
        };
        \addlegendentry{$L=40$}
        
        \end{axis}
    \end{tikzpicture}
    
    \caption{\textbf{Slepian vs.\ Spherical Harmonics on California Housing.} Dotted vertical lines denote the Shannon number for each number of Slepian Legendre polynomials. \textbf{(a)} Slepian functions show monotonic improvement up to Shannon number $N$ (dashed lines), then plateau. 
    \textbf{(b)} Spherical harmonics exhibit erratic, non-monotonic behavior regardless of embedding size.}
    \label{fig:slepian_vs_sh}
\end{wrapfigure}
